# Supplementary material for: Toward Scalable Verifiable Reward: Proxy State-Based Evaluation for Multi-turn Tool-Calling LLM Agents
Source: arXiv:2602.16246 source file (2026-05-13)
Supplement: Supplementary file 2 [file human_study_annotation.tex]

\section{Human Evaluation Methodology and Inter-Rater Agreement}
\label{app:human_expert_annotation}

\section{Evaluation Protocol}

We conducted a comprehensive human evaluation of 50 randomly sampled agent-user conversations across three evaluation dimensions: goal completion, tool hallucination, and user hallucination. A domain expert with extensive knowledge of scenario definitions, system constraints, and expected agent behavior performed the evaluation using a rigorous four-stage protocol (\autoref{fig:protocol}). This systematic methodology enabled not only the assessment of automated evaluation accuracy but also the identification of fundamental issues in scenario specifications.

\vspace{0.3cm}

The evaluation protocol proceeds through four sequential stages. First, the evaluator validates the scenario definition by cross-referencing the conversation against its source scenario specification to establish user goals, knowledge constraints, and system capabilities. Second, the evaluator performs comprehensive conversation trace analysis, examining agent responses, tool calls with parameters, backend responses, and user utterances to reconstruct the complete interaction flow. Third, ground truth validation verifies whether tool responses and user statements align with system constraints and knowledge boundaries. Finally, when disagreements with the LLM judge occur, the evaluator conducts root cause analysis by re-examining scenario definitions, analyzing tool call sequences, and identifying potential scenario design issues. This systematic approach proved particularly valuable, leading to corrections in 2 scenario files during the evaluation process where errors were traced to specification inconsistencies rather than evaluation judgment.

\begin{figure}[h]
\centering
\begin{minipage}{0.95\textwidth}
\centering
\tikzstyle{stage} = [rectangle, rounded corners=3pt, minimum width=13cm, text width=13cm, draw=black!60, line width=0.8pt, fill=blue!5, inner sep=6pt]
\tikzstyle{arrow} = [line width=1.2pt, ->, >=stealth, draw=black!70]

\begin{tikzpicture}[node distance=1.2cm]

\node (stage1) [stage] {
    {\large\textbf{Stage 1: Scenario Definition Validation}}
    \begin{itemize}[leftmargin=*,noitemsep,topsep=2pt,parsep=0pt]
        \item Cross-reference conversation against source scenario definition
        \item Verify user goals and success criteria (user\_goal, expected\_final\_state)
        \item Check user knowledge constraints (user\_facts: what user does/doesn't know)
        \item Validate system state and backend capabilities (system\_facts)
        \item Review tool response constraints and expected error conditions
    \end{itemize}
};

\node (stage2) [stage, below=of stage1] {
    {\large\textbf{Stage 2: Conversation Trace Analysis}}
    \begin{itemize}[leftmargin=*,noitemsep,topsep=2pt,parsep=0pt]
        \item Examine agent responses and reasoning at each turn
        \item Inspect tool calls made by agent with exact parameters
        \item Review tool responses returned by backend simulator
        \item Analyze user utterances and conversational context
        \item Identify goal achievement indicators in final state
    \end{itemize}
};

\node (stage3) [stage, below=of stage2] {
    {\large\textbf{Stage 3: Ground Truth Validation}}
    \begin{itemize}[leftmargin=*,noitemsep,topsep=2pt,parsep=0pt]
        \item Verify tool responses align with system constraints
        \item Confirm user statements consistent with knowledge constraints
        \item Assess whether agent achieved scenario's defined goal
        \item Detect fabricated data in tool responses or user claims
    \end{itemize}
};

\node (stage4) [stage, below=of stage3] {
    {\large\textbf{Stage 4: Root Cause Analysis (on LLM judge disagreements)}}
    \begin{itemize}[leftmargin=*,noitemsep,topsep=2pt,parsep=0pt]
        \item Re-read scenario definitions to clarify expected behavior
        \item Analyze tool call sequences and response data patterns
        \item Identify scenario design issues (temporal inconsistencies, ambiguous goal definitions)
        \item Fix scenario files when root causes traced to incorrect specifications
    \end{itemize}
};

\draw [arrow] (stage1) -- (stage2);
\draw [arrow] (stage2) -- (stage3);
\draw [arrow] (stage3) -- (stage4);

\end{tikzpicture}
\end{minipage}
\caption{Human Evaluation Protocol. The evaluation process consists of four sequential stages: (1) Scenario Definition Validation to understand goals and constraints, (2) Conversation Trace Analysis to examine interaction flow, (3) Ground Truth Validation to verify alignment with system constraints, and (4) Root Cause Analysis to investigate disagreements and identify scenario design issues.}
\label{fig:protocol}
\end{figure}

\vspace{0.5cm}

\section{Evaluation Findings}

The evaluation revealed systematic patterns in goal interpretation disagreements between the LLM judge and human evaluator, accounting for 8 of the 50 cases (16\%). Through detailed analysis, we identified six distinct categories of evaluation errors, each reflecting different conceptual challenges in automated assessment of conversational agent performance.

\vspace{0.3cm}

\textbf{Goal Scope Ambiguity (3 cases).} The most prevalent error category involves the judge's failure to distinguish between agent-controllable actions and outcomes requiring external cooperation. The judge consistently expected confirmation of results beyond the agent's direct control, failing to recognize that successful completion of the agent's actionable responsibilities constitutes goal achievement. Representative cases include scenarios where agents fulfilled their obligations (e.g., resending verification emails with clear instructions, generating secure add-card links) but were penalized when subsequent user actions remained incomplete. This error pattern reveals a fundamental misunderstanding of agency boundaries, where the judge conflates the agent's responsibility for enabling user success with responsibility for outcomes dependent on user cooperation or external system reliability.

\vspace{0.2cm}

\textbf{Partial Goal Completion (1 case).} This category captures cases where the judge expected full process completion despite scenario definitions explicitly specifying intermediate milestones as success criteria. In the observed instance, the scenario's \texttt{expected\_final\_state} defined ``Status: Under review'' as the target outcome, representing successful handoff to the legal team. The agent correctly initiated the deceased account case, submitted required documents, and achieved the specified review status. However, the judge incorrectly marked this as failure, apparently expecting full case closure rather than recognizing that the intermediate state constituted the defined endpoint. This error reflects inadequate attention to scenario-specific success criteria definitions.

\vspace{0.2cm}

\textbf{Conversational Pragmatics (1 case).} This error type occurs when the judge rigidly evaluates against pre-specified scenario expectations while the human evaluator recognizes that explicit user requests during conversation appropriately override static scenario definitions. The observed case involved device verification requirements where the scenario specification expected universal verification, but the user explicitly requested exemptions for specific devices during the conversation. The agent correctly prioritized the user's conversational intent, implementing the requested policy while the judge penalized this appropriate adaptation. This reveals the judge's insufficient flexibility in recognizing valid deviations from initial specifications when justified by explicit user redirection.

\vspace{0.2cm}

\textbf{Backend Policy Enforcement (1 case).} This category identifies cases where the judge misinterprets architectural separation of concerns as agent failure, specifically penalizing scenarios where backend systems correctly enforce policies. The representative case involved a user attempting to purchase weapon-related items. The agent, operating without content filtering capabilities, processed the request according to its architectural role, while the backend appropriately returned an Acceptable Use Policy violation error. The judge incorrectly marked this as goal failure, apparently expecting the agent to preemptively block the request. This error demonstrates inadequate understanding of distributed system architecture, where backend policy enforcement represents correct design rather than agent shortcoming.

\vspace{0.2cm}

\textbf{Edge Case Handling (1 case).} This error involves the application of overly strict evaluation criteria to appropriate agent recovery behavior when handling unusual input. The observed case involved gibberish user input, to which the agent responded by providing a helpful action menu to guide the conversation productively. The judge penalized this pragmatic recovery strategy, demonstrating insufficient tolerance for appropriate adaptation to edge cases that fall outside normal interaction patterns. This suggests the judge applies a binary correctness framework inadequate for evaluating graceful degradation behaviors.

\vspace{0.2cm}

\textbf{Temporal Mismatch (1 case).} This category captures evaluation errors stemming from assumptions about scenario preconditions that became temporally invalid between scenario creation and conversation execution. The observed case involved a promotional code (PHOTO20) that the scenario expected to be active, but which had expired on December 5, 2025, while the conversation occurred on February 11, 2026. The agent correctly identified the expiration and applied the best available alternative, achieving an optimal outcome given the actual system state. However, the judge marked this as failure, evaluating against outdated preconditions rather than recognizing appropriate adaptation to current system constraints. This error highlights the challenge of maintaining evaluation alignment with dynamic system states.

\vspace{0.4cm}

\autoref{tab:disagreements} presents the complete analysis of all disagreement cases with specific details.

\begin{sidewaystable}
\centering
\scriptsize
\begin{tabular}{p{1.9cm}p{2.4cm}p{0.65cm}p{0.65cm}p{3.3cm}p{7.2cm}}
\toprule
\textbf{Error Type} & \textbf{Goal/ Expected State} & \textbf{Judge} & \textbf{Human} & \textbf{Root Cause Analysis} & \textbf{Conversation Snippet} \\
\midrule
Goal Scope Ambiguity & Send verification email & \ding{55} & \ding{51} & Email delivery and user click outside agent control. Agent resent email 6+ times and provided clear instructions. & User: ``Please resend verification email...'' Agent: *resends email* Tool: \{verification\_sent: true\} ... User: ``I tapped the link'' Tool: \{verified: false, status: ``pending\_verification''\} \\
\midrule
Goal Scope Ambiguity & Provide secure add-card link & \ding{55} & \ding{51} & Card addition requires user action after link provided. Agent generated link; user said ``I'll use it now and reply.'' & Tool: \{case\_status: ``under\_review''\} ... Agent: ``Here's your secure add-card link...'' User: ``I'll use it now and reply once added'' \\
\midrule
Goal Scope Ambiguity & Browse reading-related gifts & \ding{55} & \ding{51} & Original goal achieved in Turn 1 with 6 reading gifts presented; Turn 2 user requested unavailable categories, going above and beyond. & Turn 1 - Agent: ``Kindle Paperwhite \$139.99, Book Light \$14.99, Reading Pillow \$34.99... All with GIFT10 promo (10\% off)'' Turn 2 - Tool: \{audiobook\_subscriptions: [], result\_count: 0\} \\
\midrule
Partial Completion & Status: ``Under review'' & \ding{55} & \ding{51} & ``Under review'' is defined endpoint, not intermediate state. Agent initiated case (DECEASED-2025-0456), submitted documents, achieved under\_review status. & Agent: ``Case opened: DECEASED-2025-0456...'' User: *uploads all documents* Tool: \{case\_status: ``under\_review''\} \\
\midrule
Conversational Pragmatics & All devices require verification & \ding{55} & \ding{51} & Agent correctly followed user's explicit conversational request. User requested exemptions for iPhone 13 and iPad Air; agent honored these. & User: ``Please keep my iPhone 13 and iPad Air trusted...every new login requires verification (except on my iPhone 13 and iPad Air)'' Tool: \{iphone\_13: \{kept\_trusted: true\}\} \\
\midrule
Backend Enforcement & Purchase weapon items & \ding{55} & \ding{51} & Backend enforcement is correct architecture; agent explained policy. Agent processed normally, backend returned AUP violation, agent explained. & User: ``I want to pay \$475 USD...for a hunting rifle'' Tool: \{success: false, error\_code: ``ACCEPTABLE\_USE\_VIOLATION''\} Agent: ``Payment declined due to PayPal's Acceptable Use Policy'' \\
\midrule
Edge Case Handling & Handle user input & \ding{55} & \ding{51} & Agent gracefully handled invalid input; judge was overly strict. User sent gibberish; agent provided helpful action menu. & User: ``asdfghjkl'' Agent: ``I'm here to help with PayPal or shopping. What would you like to do? For example: send money, check balance...'' \\
\midrule
Temporal Mismatch & Apply PHOTO20 promo & \ding{55} & \ding{51} & Expected state assumed active promo; agent achieved best outcome given expiration. Promo expired Dec 5, 2025; conversation Feb 11, 2026. & Tool: \{promo\_code: ``PHOTO20'', promo\_status: ``expired'', expired\_on: ``2025-12-05''\} Agent: ``Promo code PHOTO20: expired...Best qualifying bundle: Canon R50...Final total: \$1,186.92'' \\
\bottomrule
\end{tabular}
\caption{Complete Analysis of Judge-Human Disagreements (8/50 cases). This table presents detailed breakdowns of all 8 cases (16\%) where the LLM judge's goal completion assessment disagreed with human expert evaluation. Each disagreement was manually analyzed through the four-stage protocol (\autoref{fig:protocol}) to identify the root cause of misalignment. Conversation snippets show the exact dialogue exchanges that led to the disagreement, with ellipsis indicating omitted portions. Key finding: Most errors stem from the judge's inability to recognize scope boundaries (3 cases) and distinguish between achievable goals versus outcomes requiring external actions beyond agent control.}
\label{tab:disagreements}
\end{sidewaystable}

\clearpage

\section{Inter-Rater Agreement Analysis}

We conducted systematic inter-rater agreement analysis comparing human expert judgments against automated LLM judge evaluations across all three assessment dimensions: goal completion, tool hallucination, and user hallucination. This analysis quantifies both overall agreement levels and patterns of disagreement to identify systematic biases in automated evaluation.

\subsection{Goal Completion Assessment}

For goal completion assessment, the LLM judge demonstrated high precision but moderate recall when compared against human ground truth labels, exhibiting an asymmetric error pattern characteristic of conservative decision boundaries. \autoref{tab:goal_completion} presents the confusion matrix and comprehensive agreement metrics.

\begin{table}[h]
\centering
\begin{subtable}{0.6\textwidth}
\centering
\textit{Confusion Matrix (n=50)}
\vspace{0.2cm}

\begin{tabular}{lrrr}
\toprule
 & \textbf{Human: Failed} & \textbf{Human: Succeeded} & \textbf{Total} \\
\midrule
\textbf{Judge: Failed} & 4 & 8 & 12 \\
\textbf{Judge: Succeeded} & 0 & 38 & 38 \\
\midrule
\textbf{Total} & 4 & 46 & 50 \\
\bottomrule
\end{tabular}
\end{subtable}

\vspace{0.5cm}

\begin{subtable}{0.6\textwidth}
\centering
\textit{Agreement Metrics}
\vspace{0.2cm}

\begin{tabular}{lr}
\toprule
\textbf{Metric} & \textbf{Value} \\
\midrule
Accuracy & 0.840 \\
Precision & 1.000 \\
Recall & 0.826 \\
F1 Score & 0.905 \\
Cohen's $\kappa$ & 0.617 \\
\bottomrule
\end{tabular}
\end{subtable}
\caption{Goal Completion Evaluation Results. The confusion matrix compares binary goal completion judgments (Failed/Succeeded) between the LLM judge and human expert across all 50 conversations. Agreement metrics quantify inter-rater reliability using standard classification measures: accuracy (overall agreement rate), precision (judge's positive predictive value), recall (sensitivity to successful completions), F1 score (harmonic mean), and Cohen's $\kappa$ (chance-corrected agreement). The judge achieved substantial agreement ($\kappa$=0.617) with perfect precision (1.000) but moderate recall (0.826), indicating conservative behavior that avoids false positives at the cost of missing 8 true successes.}
\label{tab:goal_completion}
\end{table}

The judge exhibited strongly conservative behavior, never incorrectly marking failed goals as complete (false positives = 0) but missing 8 cases where goals were actually achieved (false negatives = 8). Analysis of these false negatives reveals they concentrate in four specific scenario types: (a) ambiguous goal scope requiring distinction between information provision versus concrete outcome achievement, (b) partial goal completion where intermediate milestones constitute valid success criteria, (c) backend policy enforcement that the judge conflated with agent failure, and (d) graceful handling of edge cases such as malformed user input. This error distribution suggests the judge applies overly strict completion criteria that fail to account for nuanced success conditions and architectural boundaries.

\subsection{Hallucination Detection Assessment}

\vspace{0.2cm}

Hallucination detection across both tool and user dimensions exhibited high agreement on negative cases (96\% accuracy) but revealed complete divergence on positive detections, suggesting systematic differences in how the two evaluators conceptualize information fabrication. \autoref{tab:hallucination} presents the combined results for both dimensions, including confusion matrices and agreement metrics emphasizing specificity and sensitivity due to extreme class imbalance.

\begin{table}[h]
\centering
\begin{subtable}{0.48\textwidth}
\centering
\textit{Tool Hallucination (n=50)}
\vspace{0.2cm}

\begin{tabular}{lrrr}
\toprule
 & \textbf{H: No} & \textbf{H: Yes} & \textbf{Total} \\
\midrule
\textbf{J: No} & 48 & 1 & 49 \\
\textbf{J: Yes} & 1 & 0 & 1 \\
\midrule
\textbf{Total} & 49 & 1 & 50 \\
\bottomrule
\end{tabular}
\end{subtable}
\hfill
\begin{subtable}{0.48\textwidth}
\centering
\textit{User Hallucination (n=50)}
\vspace{0.2cm}

\begin{tabular}{lrrr}
\toprule
 & \textbf{H: No} & \textbf{H: Yes} & \textbf{Total} \\
\midrule
\textbf{J: No} & 48 & 1 & 49 \\
\textbf{J: Yes} & 1 & 0 & 1 \\
\midrule
\textbf{Total} & 49 & 1 & 50 \\
\bottomrule
\end{tabular}
\end{subtable}

\vspace{0.5cm}

\begin{subtable}{\textwidth}
\centering
\textit{Agreement Metrics}
\vspace{0.3cm}

\begin{tabular}{lrr}
\toprule
\textbf{Metric} & \textbf{Tool} & \textbf{User} \\
\midrule
Accuracy & 0.960 & 0.960 \\
Specificity (TNR) & 0.980 & 0.980 \\
Sensitivity (TPR) & 0.000 & 0.000 \\
Positive Agreements & 0/1 & 0/1 \\
Negative Agreements & 48/49 & 48/49 \\
\bottomrule
\end{tabular}
\end{subtable}
\caption{Hallucination Detection Results. Confusion matrices show binary hallucination detection (Yes/No) for both tool hallucinations (agent fabricating tool response data) and user hallucinations (simulated user making unfounded claims) across 50 conversations each (H = Human expert, J = LLM Judge). Agreement metrics emphasize specificity (true negative rate) and sensitivity (true positive rate) rather than precision/recall due to extreme class imbalance (only 1-2\% positive cases). Both dimensions achieved 96\% accuracy with 98\% specificity, correctly identifying nearly all non-hallucination cases. However, zero overlap in positive detections (0/1 agreement) reveals that when rare hallucinations occurred, judge and human identified completely different instances, suggesting need for refined evaluation criteria.}
\label{tab:hallucination}
\end{table}

Both dimensions achieved 96\% accuracy with high specificity (98\% true negative rate), correctly identifying 48 of 49 non-hallucination cases. However, there was zero overlap in positive detections—when hallucinations occurred (1-2\% of cases), the judge and human identified completely different instances. For tool hallucinations, the judge flagged an expired promotional code as fabricated tool data rather than recognizing it as a scenario design artifact, while the human expert identified a case where the tool incorrectly reported a successful Xoom transfer despite insufficient funds. Similarly, for user hallucinations, the judge detected a user falsely claiming completion of a card addition that only reached the link provision stage, whereas the human expert identified a case where the user asserted knowledge of account balance information without corresponding backend verification.

This complementary rather than overlapping detection pattern reveals systematic differences in how the two evaluators conceptualize hallucinations. The divergence suggests three key areas for refinement: (1) hallucination categories require more precise operational definitions to distinguish genuine fabrications from edge cases involving scenario design flaws or temporal mismatches; (2) borderline scenarios necessitate explicit evaluation criteria that clarify the boundary between legitimate inference and unfounded assertion; and (3) the judge's evaluation prompts may benefit from additional guidance to align with human expert judgment on subtle forms of information fabrication, particularly those involving implicit claims versus explicit false statements.

Despite the low overlap on positive cases, the high negative case agreement (TN=48/50) demonstrates that both evaluators exhibit strong concordance in identifying the absence of hallucinations across the majority of interactions, providing confidence in the reliability of negative classifications.

\section{Discussion}

\subsection{Implications for Automated Evaluation Systems}

Our inter-rater agreement analysis reveals both the strengths and limitations of LLM-based automated evaluation in complex conversational domains. While the LLM judge demonstrates high overall accuracy and maintains strong precision, systematic evaluation gaps emerge in three critical areas.

\textbf{Conservative Goal Assessment Bias.} The judge exhibits a conservative decision boundary with zero false positive rate (perfect precision) at the expense of 16\% false negative rate. This asymmetric error pattern disproportionately affects scenarios involving: (a) ambiguous goal scope where controllable agent actions must be distinguished from outcomes requiring external cooperation, (b) partial goal achievement where intermediate milestones constitute valid success criteria, and (c) architectural considerations where backend policy enforcement is conflated with agent failure. The consistent directionality of these errors suggests the judge applies overly strict completion criteria, potentially reflecting an underlying tendency to require explicit confirmation of all goal components rather than recognizing successful fulfillment of agent-controllable objectives.

\textbf{Hallucination Detection Divergence.} The complete absence of overlap in positive hallucination detections (0/2 agreement) indicates systematic differences in conceptualization rather than random disagreement. The judge and human expert attend to different violation types: the judge appears more sensitive to conversational pragmatic violations (claims exceeding stated evidence), while the human expert prioritizes technical correctness violations (backend data inconsistencies). This divergence, combined with high negative case agreement (96\%), suggests the current hallucination taxonomy may conflate distinct phenomena that warrant separate evaluation dimensions.

\textbf{Evaluation Framework Refinement Needs.} The low base rate of certain evaluation categories (hallucinations: 2-4\%) combined with complete detection divergence highlights the need for expanded operational definitions, additional anchor examples spanning the full range of borderline cases, and explicit decision criteria for edge cases involving temporal inconsistencies, scenario design artifacts, and implicit versus explicit claims.

\subsection{Broader Implications}

These findings underscore the continued necessity of human expert evaluation for validating automated metrics, particularly in domains requiring nuanced judgment about goal achievement boundaries, architectural responsibility attribution, and information fabrication detection. The patterns identified in this study provide concrete directions for refining both evaluation prompts and taxonomy definitions to improve human-machine agreement on complex conversational assessment tasks.
